# Supplementary material for: Laser threshold magnetometry
Source: arXiv:1410.6239 source file (2016-01-09)
Supplement: Supplementary file 1 [file Supplementary.pdf]

# Laser threshold magnetometer - Supplementary material

Jan Jeske,[1] Jared H. Cole,[1] and Andrew D. Greentree[1]
[1] *Chemical and Quantum Physics, School of Applied Sciences, RMIT University, Melbourne 3001, Australia*

## METHOD FOR FINDING THE STEADY STATE SOLUTION OF THE EQUATIONS OF MOTION

The equations of motion for our simplified model are:

$$\begin{aligned}
\dot{\rho}_{11} &= -2\Omega\ \mathrm{Im}(\rho_{14}) - \Lambda_{12}\rho_{11} + L_{21}\rho_{22} + L_{31}\rho_{33} + L_{71}\rho_{77},\\
\dot{\rho}_{14} &= (i\Delta - \Gamma_{14} - \Lambda_{12}/2 - \Lambda_{45}/2)\rho_{14} - i\Omega\,(\rho_{44} - \rho_{11}),\\
\dot{\rho}_{22} &= \Lambda_{12}\rho_{11} - (L_{21} + L_{23})\,\rho_{22} - G_{23}\,(\rho_{22} - \rho_{33})\,n,\\
\dot{\rho}_{33} &= L_{23}\rho_{22} - L_{31}\rho_{33} - G_{23}\,(\rho_{33} - \rho_{22})\,n,\\
\dot{\rho}_{44} &= 2\Omega\ \mathrm{Im}(\rho_{14}) - \Lambda_{45}\rho_{44} + L_{54}\rho_{55} + L_{64}\rho_{66} + L_{74}\rho_{77},\\
\dot{\rho}_{55} &= \Lambda_{45}\rho_{44} - (L_{54} + L_{56} + L_{57})\,\rho_{55} - G_{56}\,(\rho_{55} - \rho_{66})\,n,\\
\dot{\rho}_{66} &= L_{56}\rho_{55} - L_{64}\rho_{66} - G_{56}\,(\rho_{66} - \rho_{55})\,n,\\
\dot{\rho}_{77} &= L_{57}\rho_{55} - (L_{71} + L_{74})\,\rho_{77},\\
\dot{n} &= G_{23}\,(\rho_{22} - \rho_{33})\,n + G_{56}\,(\rho_{55} - \rho_{66})\,n - \kappa n, \qquad (1)
\end{aligned}$$

They are nonlinear equations since $n$ is multiplied with the density matrix elements. They can therefore not be solved dynamically via diagonalisation of the superoperator. However for the steady state solution we can assume that all variables are constant (except the oscillation of the off-diagonal elements $\rho_{14}, \rho_{41}$ and therefore treat $n$ as a constant, unknown parameter in the equations of motion. We then rewrite these equations in matrix form on the next page. We then find the steady state solution by finding the nullspace. The unnormalized solution for the populations and coherences $\rho_{ij}$, as a function of $n$, is also given on the next page.

With this solution for the $\rho_{ij}(n)$ we can then write down the remaining equation for $n$. To do so we normalise the solution first by dividing the solution by $\sum_{j=1}^{7} \rho_{jj}$. We then insert the normalised steady state solutions for the $\rho_{ij}(n)$ into eq. 1. As we are interested in the steady state we set $\dot{n} = 0$ in the equation:

$$0 = G_{23}\,(\rho_{22} - \rho_{33})\,n + G_{56}\,(\rho_{55} - \rho_{66})\,n - \kappa n \qquad (2)$$

Note that this has the solution $n = 0$ because we neglected spontaneous emission in the equation. We are interested in the non-zero solution of the equation:

$$0 = G_{23}\,(\rho_{22} - \rho_{33}) + G_{56}\,(\rho_{55} - \rho_{66}) - \kappa \qquad (3)$$

This equation has two solutions for $n$, one of which is purely negative and unphysical. We obtained the other solution, however the long expression is unhelpful to be written down explicitly here. It gives the equilibrium value for $n$ as a function of all system parameters.

To consider the four orientations, where the magnetic field is aligned along one, the aligned and misaligned directions are treated with separate density matrices and contribute to eq. 1 with 1/4 and 3/4 respectively.

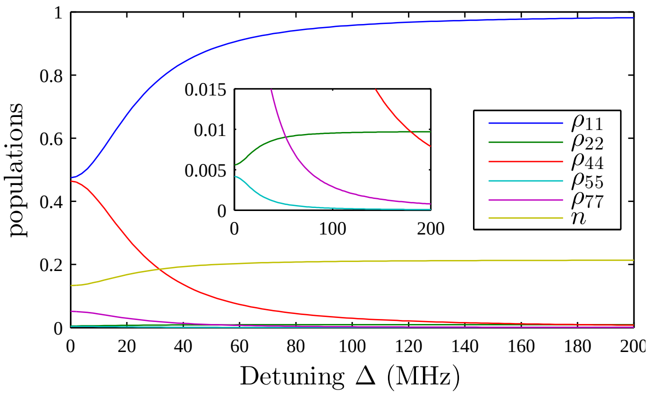


FIG. 1. Populations of the levels in the steady state as a function of detuning $\Delta$ for a pumping of $\Lambda = 1.5$MHz, that is above both lasing thresholds ($\kappa = 3$MHz, $\Omega = 3.67$MHz). One can see the transition from lasing with populations in spin 0 and spin 1 states (resonant Rabi driving) to lasing with populations only in the spin 0 manifold (off-resonant Rabi driving). The inset shows the curves with very low populations.

## LASING POPULATIONS PLOT

Figure 1 shows the steady state populations as a function of the detuning for a laser pumping rate above the operating point, i.e. above the lasing threshold even for large detuning ($n > 0$ in the entire plot). It shows that with increasing detuning, the populations of the spin 1 manifold ($\rho_{44}, \rho_{55}, \rho_{77}$) are reduced to zero; lasing occurs with spin 0 states only and the signal $n$ becomes stronger.

## RESPONSE TIME PLOTS

Figure 2 shows numerical simulations of how quickly the device adapts to sudden changes of the magnetic field at $t = 0$ in each plot. In the right column the new equilibrium state is reached after about 30$\mu$s; the parameters correspond to the yellow dashed line in figure 2 of the main text. In the left column the response time is much faster, parameters correspond to the blue line in figure 3 of the main text. While the cavity photon number $n$ determines the equilibration of the laser output, the populations of states $|1\rangle$ and $|4\rangle$ give insight into the equilibration process between the spin manifolds. A spontaneous emission rate of 1kHz into the cavity from $|2\rangle$ and $|5\rangle$ was considered in all simulations.

$$
\begin{pmatrix} \dot\rho_{14} \\ \dot\rho_{41} \\ \dot\rho_{11} \\ \dot\rho_{22} \\ \dot\rho_{33} \\ \dot\rho_{44} \\ \dot\rho_{55} \\ \dot\rho_{66} \\ \dot\rho_{77} \end{pmatrix}
=
\begin{pmatrix}
\alpha+i\Delta & 0 & i\Omega & 0 & 0 & -i\Omega & 0 & 0 & 0 \\
0 & \alpha-i\Delta & -i\Omega & 0 & 0 & i\Omega & 0 & 0 & 0 \\
i\Omega & -i\Omega & -\Lambda_{12} & L_{21} & L_{31} & 0 & 0 & 0 & L_{71} \\
0 & 0 & \Lambda_{12} & -L_{21}-L_{23}-G_{23}n & G_{23}n & 0 & 0 & 0 & 0 \\
0 & 0 & 0 & L_{23}+G_{23}n & -L_{31}-G_{23}n & 0 & 0 & 0 & 0 \\
-i\Omega & i\Omega & 0 & 0 & 0 & -\Lambda_{45} & L_{54} & L_{64} & L_{74} \\
0 & 0 & 0 & 0 & 0 & \Lambda_{45} & -L_{54}-L_{56}-L_{57}-G_{56}n & G_{56}n & 0 \\
0 & 0 & 0 & 0 & 0 & 0 & L_{56}+G_{56}n & -L_{64}-G_{56}n & 0 \\
0 & 0 & 0 & 0 & 0 & 0 & L_{57} & 0 & -L_{71}-L_{74}
\end{pmatrix}
\begin{pmatrix} \rho_{14} \\ \rho_{41} \\ \rho_{11} \\ \rho_{22} \\ \rho_{33} \\ \rho_{44} \\ \rho_{55} \\ \rho_{66} \\ \rho_{77} \end{pmatrix}
$$

with $\alpha = -\Gamma_{14} - \frac{\Lambda_{12}}{2} - \frac{\Lambda_{45}}{2}$ and $\beta = \Lambda_{12} + \Lambda_{56}$

$$
\begin{pmatrix}
\frac{iL_{71}(\beta+2\Gamma_{14}+2i\Delta)}{2(\beta+2\Gamma_{14})\Omega} \\
-\frac{iL_{71}(\beta+2\Gamma_{14}-2i\Delta)}{2(\beta+2\Gamma_{14})\Omega} \\
\frac{4(L_{71}+L_{74})(L_{64}(L_{56}+G_{56}n)+L_{54}(L_{64}+G_{56}n))(\beta+2\Gamma_{14})\Omega^2+L_{57}(L_{64}+G_{56}n)\left(4L_{74}(\beta+2\Gamma_{14})\Omega^2+L_{71}\left(\beta^2\Lambda_{45}+4\beta\left(\Gamma_{14}\Lambda_{45}+\Omega^2\right)+4\left(\Gamma_{14}^2\Lambda_{45}+\Delta^2\Lambda_{45}+2\Gamma_{14}\Omega^2\right)\right)\right)}{4L_{57}(L_{64}+G_{56}n)(\beta+2\Gamma_{14})\Lambda_{45}\Omega^2} \\
\frac{(L_{31}+G_{23}n)\Lambda_{12}\left(4(L_{71}+L_{74})(L_{64}(L_{56}+G_{56}n)+L_{54}(L_{64}+G_{56}n))(\beta+2\Gamma_{14})\Omega^2+L_{57}(L_{64}+G_{56}n)\left(4L_{74}(\beta+2\Gamma_{14})\Omega^2+L_{71}\left(\beta^2\Lambda_{45}+4\beta\left(\Gamma_{14}\Lambda_{45}+\Omega^2\right)+4\left(\Gamma_{14}^2\Lambda_{45}+\Delta^2\Lambda_{45}+2\Gamma_{14}\Omega^2\right)\right)\right)\right)}{4L_{57}(L_{64}+G_{56}n)(L_{31}(L_{23}+G_{23}n)+L_{21}(L_{31}+G_{23}n))(\beta+2\Gamma_{14})\Lambda_{45}\Omega^2} \\
\frac{(L_{23}+G_{23}n)\Lambda_{12}\left(4(L_{71}+L_{74})(L_{64}(L_{56}+G_{56}n)+L_{54}(L_{64}+G_{56}n))(\beta+2\Gamma_{14})\Omega^2+L_{57}(L_{64}+G_{56}n)\left(4L_{74}(\beta+2\Gamma_{14})\Omega^2+L_{71}\left(\beta^2\Lambda_{45}+4\beta\left(\Gamma_{14}\Lambda_{45}+\Omega^2\right)+4\left(\Gamma_{14}^2\Lambda_{45}+\Delta^2\Lambda_{45}+2\Gamma_{14}\Omega^2\right)\right)\right)\right)}{4L_{57}(L_{64}+G_{56}n)(L_{31}(L_{23}+G_{23}n)+L_{21}(L_{31}+G_{23}n))(\beta+2\Gamma_{14})\Lambda_{45}\Omega^2} \\
\frac{(L_{71}+L_{74})(L_{56}L_{64}+L_{57}L_{64}+G_{56}L_{57}n+G_{56}L_{64}n+L_{54}(L_{64}+G_{56}n))}{L_{57}(L_{64}+G_{56}n)\Lambda_{45}} \\
\frac{L_{71}+L_{74}}{L_{57}} \\
\frac{(L_{71}+L_{74})(L_{56}+G_{56}n)}{L_{57}(L_{64}+G_{56}n)} \\
1
\end{pmatrix}
$$

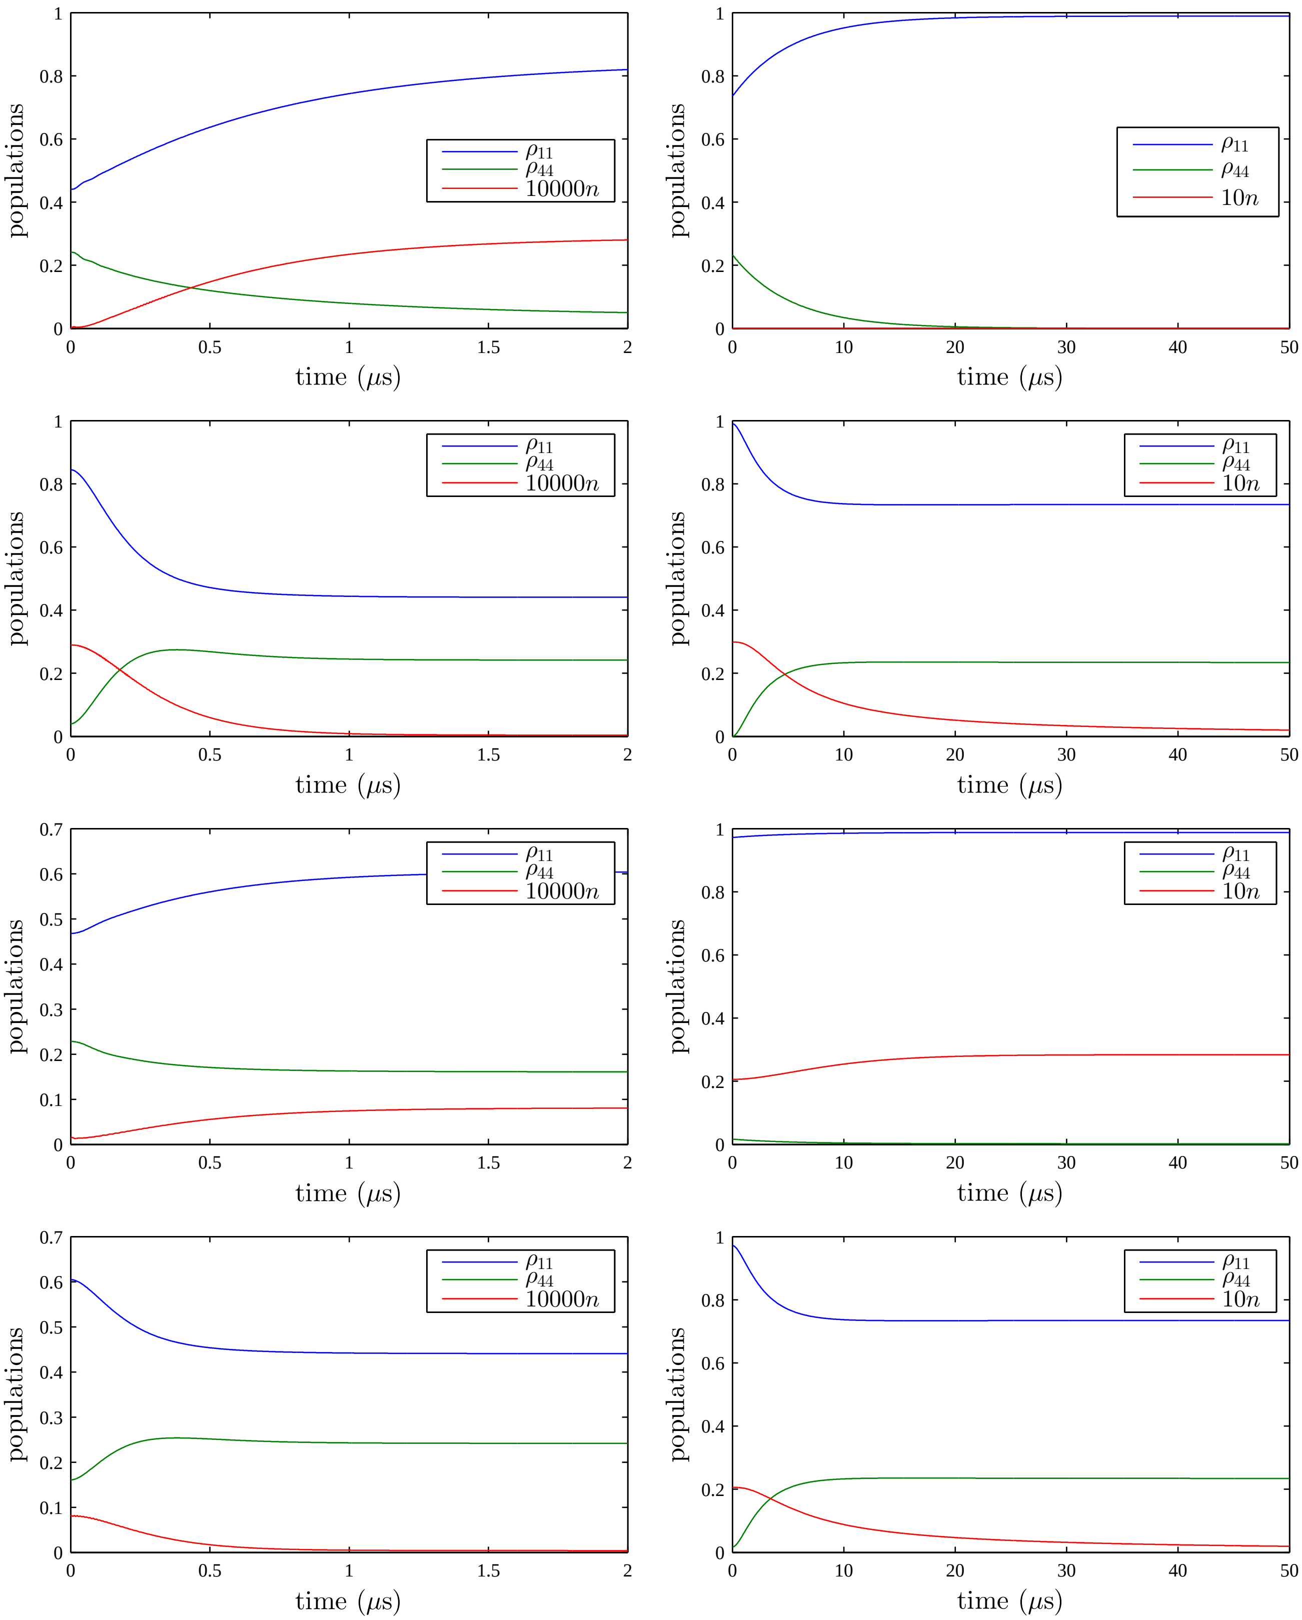


FIG. 2. Time evolution of the state populations and $n$ after an instant change of the detuning $\Delta$. The detuning changes at $t = 0$ from top to bottom: $0 \to 100$MHz, 100MHz $\to 0$, 10MHz $\to$ 30MHz, 10MHz $\to 0$. Left: For the paremeters of the blue line in Fig. 3 of the main paper, $\kappa = 63.1$GHz, $\Omega = 6.14$MHz, $\Lambda = 10.4$MHz the device takes about 2$\mu$s to reach to the new steady state. Right: For the parameters of the yellow dashed line in Fig. 3 in the main paper, $\kappa = 3$MHz, $\Omega = .367$MHz, $\Lambda = 0.940$MHz the response time is slower due to a slower laser pumping rate $\Lambda$.
